# Supplementary material for: Sci-MMR: Benchmarking Multi-Step Evidence-Grounded Scientific Reasoning in Multimodal Agents
Source: arXiv:2609.11243 source file (2026-09-22)
Supplement: Supplementary file 1 [file supp_rq1_stratified_accuracy.tex]

% Generated by build_supplementary_material.py; do not edit values manually.
\begin{table*}[!t]
\centering
\scriptsize
\setlength{\tabcolsep}{5.0pt}
\begin{tabular}{lrrrrrrr}
\toprule
Model & Bio. & Chem. & Comp. & Phys. & Hard & Med. & Easy \\
\midrule
GPT-5.5 & 54.0 & 76.5 & 73.0 & 68.2 & 29.6 & 81.5 & 96.8 \\
Claude Opus 4.8 & 48.0 & 76.5 & 61.9 & 45.5 & 11.1 & 66.3 & 95.2 \\
Kimi K2.7 & 46.0 & 55.9 & 58.7 & 45.5 & 11.1 & 56.5 & 93.5 \\
Gemini 3.1 Pro & 46.0 & 61.8 & 49.2 & 48.9 & 9.9 & 58.7 & 90.3 \\
MiniMax-M3 & 46.0 & 58.8 & 46.0 & 39.8 & 4.9 & 48.9 & 93.5 \\
GLM-5V Turbo & 46.0 & 50.0 & 36.5 & 38.6 & 8.6 & 41.3 & 83.9 \\
Qwen3.7 Plus & 40.0 & 41.2 & 33.3 & 21.6 & 4.9 & 28.3 & 71.0 \\
Intern-S2 & 30.0 & 32.4 & 23.8 & 25.0 & 4.9 & 16.3 & 71.0 \\
\midrule
\textbf{Pooled} & 44.5 & 56.6 & 47.8 & 41.6 & 10.6 & 49.7 & 86.9 \\
\bottomrule
\end{tabular}
\caption{Direct Visual Reasoning accuracy (\%) by scientific discipline and difficulty defined from Direct Visual Reasoning.}
\label{tab:supp_rq1_stratified}
\end{table*}
